# Supplementary material for: Distinguishing thixotropy, anti-thixotropy, and viscoelasticity using hysteresis
Source: arXiv:2212.07572 ancillary file (2022-12-16)
Supplement: Supplementary file 1 [file Hysteresis_SI_20221213.pdf]

APS/123-QED

# Distinguishing thixotropy, anti-thixotropy, and viscoelasticity using hysteresis

Yilin Wang

*Department of Mechanical Science and Engineering,*
*University of Illinois Urbana-Champaign, Urbana, Illinois 61801, USA*
*Beckman Institute for Advanced Science and Technology,*
*University of Illinois Urbana-Champaign, Urbana, Illinois 61801, USA and*
*Joint Center for Energy Storage Research,*
*Argonne National Laboratory, Lemont, Illinois 60439, USA*

Randy H. Ewoldt*

*Department of Mechanical Science and Engineering,*
*University of Illinois Urbana-Champaign, Urbana, Illinois 61801, USA*
*Beckman Institute for Advanced Science and Technology,*
*University of Illinois Urbana-Champaign, Urbana, Illinois 61801, USA and*
*Joint Center for Energy Storage Research,*
*Argonne National Laboratory, Lemont, Illinois 60439, USA*

(Dated: December 14, 2022)

* Author to whom correspondence should be addressed;ewoldt@illinois.edu

**Protorheology estimate of the yield stress of Laponite and carbon black (CB) suspensions**

The yield stress can be estimated based on the photographs shown in Fig. S1(a), a type of protorheology experiment as described by Hossain and Ewoldt [1].

From the photo of the Laponite suspension, the radius of the Laponite slump $R$ is around 1 cm, the height is 0.5 cm. The yield stress of Laponite suspension can be estimated by the slump test method [1]

$$\tau_y = \frac{225\rho g \Omega^2}{128\pi^2 R^5}, \tag{1}$$

where $\rho$ is the density of the suspension, which is around 1000 kg/m$^3$, $g$ is the gravitational force per unit mass, $R$ is the slump radius after slump test, and $\Omega$ is the volume of the slump. The volume is estimated by assuming a cylinder,

$$\Omega = \pi R^2 H, \tag{2}$$

where $H$ is the slump height. Taking $R = 1$ cm and $H = 0.5$ cm gives the estimated yield stress of Laponite suspension to be 43 Pa. It should be noted that the yield stress calculated in this way is expected to be a lower-bound estimate, meaning the true yield stress is at least 43 Pa. However, the proto-rheology photo of the Laponite is with an aged sample wittout sufficient pre-shear, so the estimated yield stress might be higher. From the hysteresis tests with the longest ramping time (200 s) as shown in Fig. 11(a), the yield stress of the Laponite suspension is between 20 to 30 Pa.

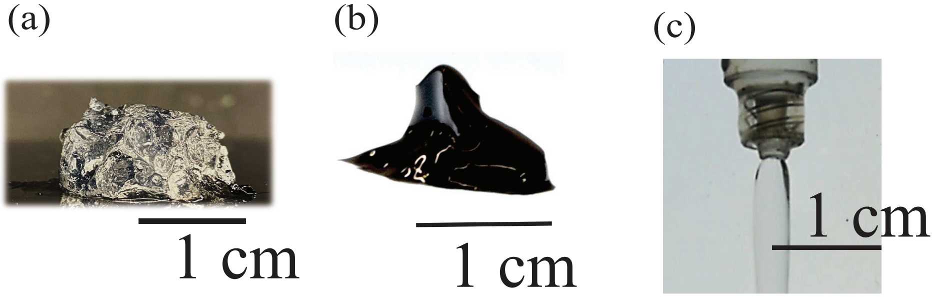


FIG. 1. Proto-rheology photos of (a) 3 wt% Laponite suspension, the estimated yield stress from the photo is 43 Pa; (b) 8 wt% carbon black suspension, the estimated yield stress is 64 Pa and (c) 1 wt% 8M PEO solution, the relaxation time of which is estimated to be 0.02 s.

For the CB suspension, the shape of the slump can no longer be approximated as a cylinder as the radius of the top of the slump is much smaller than that at the bottom.

Therefore, the inclined plane method with von Mises yield criteria is used to estimate the yield stress [1]

$$\tau_y = \rho g h \sqrt{(\sin^2\theta + \frac{1}{3}\cos^2\theta)}, \tag{3}$$

where $h$ is the height of the slump, which is 1 cm estimated form the photo; $\theta$ is the angle of the inclined plane, which is zero in this case; the density of the material $\rho$ is around 1200 kg/m$^3$. Therefore, the yield stress estimate of CB suspension is calculated to be 68 Pa. This is consistent with our previously reported measurement of apparent yield stress from steady shear measurements, which we found to be 64 Pa [2].

### Protorheology estimate of the relaxation time of the PEO solution

The nonlinear viscoelasticity of PEO solution, in particular the elastic normal stress in shear, is demonstrated by the die swell shown in the protorheology photo in Fig. S1(c). The relaxation timescale at the applied flow conditions, $\lambda(\dot{\gamma})$, can be estimated by the die swell video shown in the SI , by making several simplifying assumptions. First, we estimate the flow conditions (shear rate) of the die swell observation. From the video, we can see that the total volume, $V = 3$ mL of PEO solution was extruded from the syringe in around $t = 6$ s. This gives a volumetric flow rate, $Q = V/t$, of 0.2 mL/s. The diameter of the syringe opening, $d = 2$ mm. Assuming a parabolic velocity profile as a baseline estimate, consistent with fully-developed Newtonian pipe flow, the wall shear rate can be calculated as [3]

$$\dot{\gamma}_w = \frac{4}{\pi}\frac{Q}{(d/2)^3}. \tag{4}$$

Substituting for $Q$ and $d$, we get $\dot{\gamma}_w \approx 640$ s$^{-1}$. The true wall shear rate might be even larger for the PEO solution, which is a shear-thinning fluid.

The first normal stress difference, $N_1$, can be estimated using the die swell [3, 4]

$$N_1 = 2\sqrt{2}\tau_w\sqrt{\left(\frac{D}{d}\right)^6 - 1} \tag{5}$$

where $\tau_w$ is the wall shear stress, $D$ is the jet diameter, which is 4 mm in the video. The wall shear stress is unknown from the video, but it can be calculated by

$$\tau_w = \eta\dot{\gamma}_w, \tag{6}$$

where $\dot{\gamma}_w$ is the shear rate at wall, which is estimated using Eq. 4; $\eta$ is the shear viscosity at the applied flow (shear rate) condition. We cannot calculate the value of the shear normal stress without knowing the wall shear stress, or the shear viscosity, but we can calculate an estimate of the relaxation time without knowing that information, as follows.

The first normal stress difference is related to the viscosity and relaxation time in a few models, e.g. the White-Metzner model [5] by

$$N_1 = 2\eta(\dot{\gamma})\lambda(\dot{\gamma})\dot{\gamma}^2, \tag{7}$$

where $\eta(\dot{\gamma})$ and $\lambda(\dot{\gamma})$ are the viscosity and relaxation time at a given shear rate condition respectively. The relation (Eq. 7) reduces to

$$N_1 = 2\eta_0\lambda\dot{\gamma}^2 \tag{8}$$

for the Oldroyd-B and the second-ordered fluid models, where $\eta_0$ and $\lambda$ are constant.

Using Eq. (5), (6) and (7), we can get the relaxation time at the applied wall shear rate

$$\lambda(\dot{\gamma}_w) = \frac{\sqrt{2}}{\dot{\gamma}_w}\sqrt{\left(\frac{D}{d}\right)^6 - 1}. \tag{9}$$

Substituting values for $D/d$ and $\dot{\gamma}_w$, we can get the relaxation time under the die swell flow condition, $\lambda(\dot{\gamma}_w) \approx 0.02$ s.

Compared to the characteristic timescales we got from hysteresis tests (the ramping time when the area of hysteresis loops is maximized), which is around 1 s for the linear shear rate range (0.03 to 0.3 $s^{-1}$) and 0.4 s for the nonlinear range (0.03 to 3 $s^{-1}$), the relaxation time inferred from the die swell test is lower by more than one order of magnitude. This is as expected as the relaxation time of the PEO solution is not a constant but depends on the flow conditions. In the die swell test, the wall shear rate is $\dot{\gamma}_w = 640$ $s^{-1}$, which is much larger than the shear rate applied in hysteresis, suggesting that the flow is in an extreme nonlinear regime in the die swell. The nonlinearity can be quantified using the elastic Weissenberg number, Wi, where [5]

$$\text{Wi} = \frac{N_1}{2\tau_w} = \sqrt{2}\sqrt{\left(\frac{D}{d}\right)^6 - 1} = 11.2 \tag{10}$$

for the die swell flow. The relaxation time from die swell is an approximation and several non-ideal aspects should be noted. This includes the unsteady flow rate, small bubbles trapped in the sample, and the assumption of fully-developed flow in the (short) small diameter nozzle of the syringe. If the flow is not fully developed, then the swollen diameter, $D$, is not as large as expected from Eq.(5), and the relaxation time would be underestimated. Comparing the flow time in the syringe and the relaxation time of the sample can help resolve this concern.

In short, the die swell provides evidence for viscoelastic effects in the PEO solution, and we can quantitatively estimate the relaxation time using die swell. The result is lower but consistent with the characteristic timescale we found by hysteresis. Protorheology is not intended to replace rheometry, but is used here to provide convincing visual evidence for the presence of viscoelasticity in the PEO solution and corroborating evidence for the apparent relaxation time observed in the hysteresis tests.

### Hysteresis protocol and deviation

The continuous and discrete hysteresis with different numbers of points per decade of shear rate at different dimensionless ramping times, $T^* = 0.01$, 1, and 5 are shown in Fig. S2, 2, and S3 respectively. The corresponding deviations are calculated and plotted in Fig. S4.

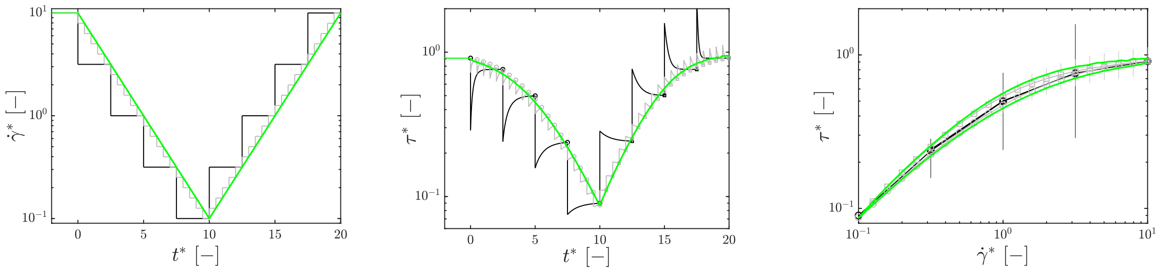


(a) (b) (c)

FIG. 2. Schematics of the step shear rate protocol to generate hysteresis loops for $T^* = n\delta t^* = 5$. (a) Input shear scheduling protocol for $n = 2$ (black), $n = 10$ (grey), and continuous shear input (green), the total time per decade is $T^* = n\delta t^* = 5$; before time zero, the shear rate is kept at the maximum value, which is 10 in this case. (b) The resulting stress response for structure based thixotropic model (Eq. 12): at each shear rate, the stress increases with time and the stress at the end of each step is chosen to be the stress at the shear rate. (c) Processing the data into hysteresis loop, the open circle shows the stress at the end of each step in the downward ramping and the open square shows those in the upward ramping, the vertical lines extending below and above the data show the transient stress during the ramping.

The total deviation $\epsilon$ is calculated as

$$\epsilon = \sum_{i=1}^{i=N} \left( \frac{\tau_i^* - \tau_{\text{con}}^*}{\tau_{\text{con}}^*} \right)^2, \tag{11}$$

where $N$ is the total number of points (for both ramping down and ramping up), $\tau_i^*$ is the stress calculated at each shear rate, and $\tau_{\text{con}}^*$ is the shear stress at the corresponding shear rate in continuous ramping.

The average deviation, $\bar{\epsilon}$, is therefore calculated as the total deviation divided by the total number of points:

$$\bar{\epsilon} = \frac{\epsilon}{N} \tag{12}$$

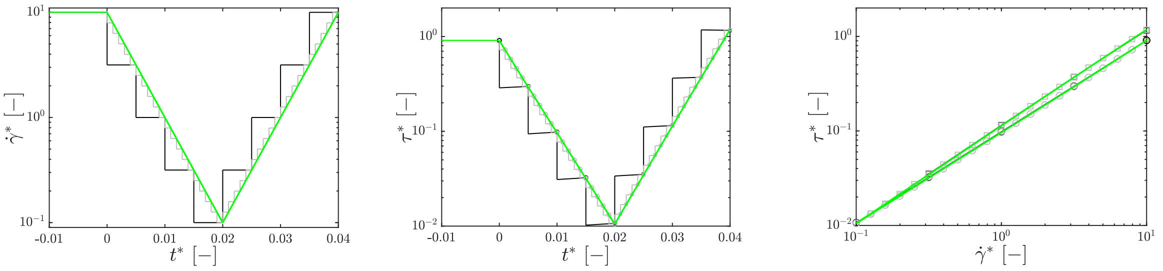


(a) (b) (c)

FIG. 3. Schematics of the step shear rate protocol to generate hysteresis loops for $T^* = n\delta t^* = 0.01$. (a) Input shear scheduling protocol for $n = 2$ (black), $n = 10$ (grey), and continuous shear input (green), the total time per decade is $T^* = n\delta t^* = 0.01$; before time zero, the shear rate is kept at the maximum value, which is 10 in this case. (b) The resulting stress response schematics for thixotropy: at each shear rate, the stress increases with time and the stress at the end of each step is chosen to be the stress at the shear rate. (c) Processing the data into hysteresis loop.

The average deviations for different $T^* = 0.01$, 1, and 5 are plotted as a function of number of points per decade of shear rate, $n$, as shown in Fig. 4.

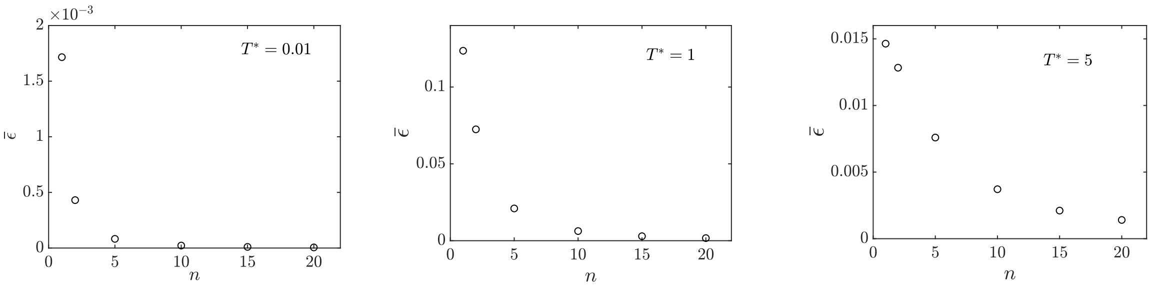


(a) (b) (c)

FIG. 4. The hysteresis calculated by discrete ramping is approaching continuous ramping with increasing number per decade. Average deviation from the continuous ramping for discrete ramping with different number per decade, the total time per decade, $T^*$ is (a) 0.01, (b) 1, and (c) 5.

Fig. S5 shows the change of thixotropic structure parameter, $\xi$, during hysteresis at $T^* = 0.001$, 0.4, and 10. The structure parameter remains nearly a constant at quick ramping ($T^* = 0.001$), increases during ramping down at the intermediate ramping time ($T^* = 0.4$), and reaches steady state at every shear rate when then ramping time is large enough ($T^* = 10$).

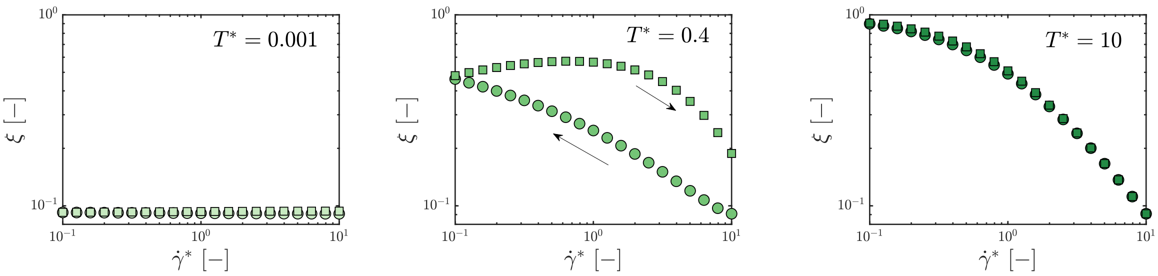


(a) (b) (c)

FIG. 5. Structure parameter during hysteresis (ramping high-low-high in $\dot{\gamma}^*$) for the thixotropic model with the ramping time $T^*$ (a) 0.001, (b) 0.04, and (c) 10.

[1] T. Hossain and R. H. Ewoldt. Proto-rheology, the first thing to do. *in preparation*.

[2] Y. Wang and R. H. Ewoldt. New insights on carbon black suspension rheology – anisotropic thixotropy and anti-thixotropy. *J. Rheol.*, 66(5):937–953, 2022.

[3] C. W Macosko. *Rheology: principles, measurements, and applications*. VCH Publishers. Inc., New York, 1994.

[4] R. H. Ewoldt and C. Saengow. Designing complex fluids. *Annu. Rev. Fluid Mech.*, 54:413–441, 2022.

[5] R. B. Bird, R. C. Armstrong, and O. Hassager. *Dynamics of Polymeric Liquids, Volume 1: Fluid mechanics, 2nd ed.* John Wiley & Sons, Inc., New York, 1987.
